# Supplementary material for: Configuration spaces on a wedge of spheres and Hochschild-Pirashvili homology
Source: arXiv:2202.12494 source file (2023-04-20)
Supplement: Supplementary file 1 [file Appendix_Hochschild.tex]

\section{Résumé of higher Hochschild homology}

We give here a brief introduction to higher Hochschild homology and to the notation used in this paper. We also recall a few useful results.

We first briefly recall the classical Hochschild homology, for $\kk$ a commutative ring.

\begin{defi}
    Let $A$ be an associative $\kk$-algebra which is a projective $\kk$-module and $M$ be an $A$-bimodule. The \emph{Hochschild complex} of the pair $(A, M)$ is the simplicial complex with objects
    \[
        C_n(A, M) = M\otimes A^{\otimes n}
    \]
    and face maps
    \begin{eqnarray}
        d_0(m\otimes a_1\otimes\ldots\otimes a_n) &= &ma_1\otimes a_2\otimes \otimes a_n\\
        d_i(m\otimes a_1\otimes\ldots\otimes a_n) &= &m \otimes a_1\otimes \ldots\otimes a_ia_{i+1}\otimes \ldots\otimes a_n\\
        d_n(m\otimes a_1\otimes\ldots\otimes a_n) &= &a_nm\otimes a_1\otimes\ldots\otimes a_{n-1}.
    \end{eqnarray}
    
    The \emph{Hochschild homology} $HH_{\ast}(A, M)$ is defined as the homology of the chain complex associated to $C_{\ast}(A, M)$ under the Dold-Kan correspondence.
\end{defi}

\begin{rmk}
    Dualizing the previous definition, one obtains similarly the Hochschild cohomology $HH^{\ast}(C, M)$ of a coalgebra $C$ and a comodule $M$.
\end{rmk}

The notion of Hochschild homology has been generalized in different directions. One of them is the notion of \emph{topological Hochschild homology}, where the algebra $A$ is replace by a ring spectrum. We will not discuss this generalization here.
What we will discuss in the rest of this section is the notion of higher Hochschild homology.

\begin{defi}[Loday construction]
    If we assume that the algebra $A$ is commutative, we can define the \emph{Loday construction} $\Loday{A}{M}$, which is the following functor $\Fin_{\ast}\to \kk-mod$
    \begin{equation*}
        \Loday{A}{M}(n_{+}) = M\otimes A^{\otimes n}.
    \end{equation*}
\end{defi}

Now if $X$ is a pointed simplicial such that the set of $p$-simplices $X_p$ is finite for all $p$, i.e. a functor $\Delta^{op}\to \Fin_{\ast}$, then for any functor $F\colon \Fin_{\ast} \to \kk-mod$, the composition $F\circ X$ is a simplicial complex.

\begin{defi}[higher Hochschild homology]
    Let $X$ be a pointed a simplicial set with finitely many $p$-simplices $X_p$ for all $p$ and $F$ be a functor $F\colon \Fin_{\ast}\to \kk-mod$. We define the higher Hochschild homology $HH_{\ast}(X, F)$ as the homology of the chain complex associated to the simplicial complex $F\circ X$ by the Dold-Kan correspondence.
\end{defi}

The interest of this definition lies in the following result:
\begin{prop}
    For any commutative $\kk$-algebra $A$ and any $A$-module $M$, there is an isomorphism
    \[
        HH_{\ast}(A, M) = HH_{\ast}(S^1, \Loday{A}{M}),
    \]
    "natural in $A$ and $M$".
\end{prop}

So the higher Hochschild homology is a generalization of the classical Hochschild homology.

\subsection{Pointed vs unpointed setting}
We defined higher Hochschild homology for a pointed simplicial set $X$ and a functor $F\colon \Fin_{\ast}\to\kk-mod$. Alternatively, for a functor $F\colon \Fin\to \kk-mod$ and an (unpointed) simplicial set $X\colon\Delta^{op}\to \Fin$ we can also define $HH_{\ast}(X, F)$ as the homology associated with the simplicial complex $F\circ X$.

\begin{defi}[reduced Loday construction]
    For an augmented $\kk$-algebra $A$, we define the \emph{reduced Loday construction} $\mathcal{L}'(A)\colon \Fin\to \kk-mod$ by
    \[
        \mathcal{L}'(A)(n) = A^{\otimes n}.
    \]
    In particular $\mathcal{L}'(A) = \kk$. 
\end{defi}

The forgetful functor $\vartheta \Fin_{\ast}\to \Fin$ admits a left adjoint $(-)_{+}\colon \Fin\to \Fin_{\ast}$. On objects, they act as follows. Let $\underline{n}_{+} = \{\ast,1,2,\ldots, n\}\in \Fin_{\ast}$ and $\underline{n} = \{1,2,\ldots, n\} \in \Fin$. Then $\vartheta(\underline{n}_{+}) = \underline{n}$, the set obtained by forgetting the basepoint, and the left adjoint $(-)_{+}$ simply adds a basepoint.

This adjunction induces by precomposition an adjunction between functor categories
\begin{equation}
    \vartheta^{\ast}\colon \mathcal{F}(\Fin, \kk) \to \mathcal{F}(\Fin_{\ast}, \kk)\colon \vartheta^{+}.
\end{equation}

This adjunction acts on the Loday constructions as follows.
\begin{lem}[Lemma 13.11, \cite{PV18}]\label{iso-Loday-constructions}
    \begin{enumerate}
        \item There is a natural isomorphism $\vartheta^{\ast}\mathcal{L}'(A) \cong \Loday{A}{A}$ in $\mathcal{F}(\Gamma, \kk)$.
        \item If $A$ is augmented, there is a natural isomorphism $\vartheta^{+}(\Loday{A}{\kk})\cong \mathcal{L}'(A)$ in $\mathcal{F}(\Fin, \kk)$. In particular we have therefore an isomorphism $\vartheta^{\ast}\vartheta^{+}(\Loday{A}{\kk} \cong \Loday{A}{A}$
    \end{enumerate}
\end{lem}

Similarly, on the level of simplicial sets we have an adjunction
\begin{equation}
    \vartheta_{+}\colon \mathcal{F}(\Delta^{op}, \Fin) \to \mathcal{F}(\Delta^{op}, \Gamma)\colon \vartheta_{\ast}.
\end{equation}

We want to understand the effect of these various adjunctions on higher Hochschild homology. Let $X\colon \Delta^{op}\to \Fin$ be an unpointed simplicial set, $Y\colon \Delta^{op}\to \Gamma$ be a pointed simplicial set and $F\in \mathcal{F}(\Fin, \kk)$ and $G\in \mathcal{F}(\Gamma, \kk)$ be two functors. What can we say about the Hochschild homology groups
\[
    HH_{\ast}(X, \vartheta^{+}(G)),\ HH_{\ast}(Y, \vartheta^{\ast}(F)),\ HH_{\ast}(\vartheta_{+}(X), G),\ HH_{\ast}(\vartheta_{\ast}(Y), F)
\]
or possibly even more interestingly of
\[
    HH_{\ast}(\vartheta_{+}(X), \vartheta^{\ast}(F)),\quad HH_{\ast}(\vartheta_{\ast}(Y), \vartheta^{+}(G)).
\]
